# Supplementary material for: Generative Temporal Models with Memory
Source: arXiv:1702.04649 source file (2017-02-21)
Supplement: Supplementary file 1 [file appendix.tex]

\section*{Appendix}
\subsection{Pseudocode for Synthetic Sequences}
\subsubsection{Perfect Recall Task}
\begin{algorithm}
  \caption{Generative Process for Perfect Recall Task}\label{pseudoPerfectRecall}
  \begin{algorithmic}[1]
    \Procedure{PerfectRecall}{\textit{dataset}}\Comment{\small{Generator for Perfect Recall}}
      \State $\textit{generator} \gets \text{sample generator for \textit{dataset}}$
	  \State $\textit{randomSeqLength} \gets \text{length of random sequence}$
      \State $\textit{first} \gets \text{\textit{first} index for the recall interval}$
      \State $\textit{last} \gets \text{\textit{last} index for the recall interval}$
      \State $\textit{sequence} \gets  \{\}$
      \\
      \For{{$i = 1,$ \textit{randomSeqLength}}}\Comment{\small{Randomly sample from the dataset}}
         \State \textit{sequence}$[i]$ $\gets s$ $\sim$  \textit{generator}$()$ 
      \EndFor
      \For{$j = $ \textit{first}, \textit{last}}
        \State append(\textit{sequence}, \textit{sequence}$[j]$) \Comment{\small{Repeat samples from recall interval}}
      \EndFor
      \State \textbf{return} \textit{sequence}\Comment{\small{Return full sequence}}
    \EndProcedure
  \end{algorithmic}
\end{algorithm}

\subsubsection{Even-Odd Transition Task}
\begin{algorithm}
  \caption{Generative Process for Even-Odd Transition Task}\label{pseudoEvenOdd}
  \begin{algorithmic}[1]
    \Procedure{EvenOddTransition}{\textit{dataset}}\Comment{\small{Generator for Even-Odd Transition}}
      \State $\textit{generator} \gets \text{sample generator for \textit{dataset}}$
	  \State $\textit{randomSeqLength} \gets \text{length of random sequence}$
      \State $\textit{first} \gets \text{\textit{first} index for the recall interval}$
      \State $\textit{last} \gets \text{\textit{last} index for the recall interval}$
      \State $\textit{sequence}, \textit{labels} \gets  \{\}, \{\}$
      \\
      \For{{$i = 1,$ \textit{randomSeqLength}}}  \Comment{\small{Randomly sample from the dataset}}
         \State \textit{sequence}$[i]$, \textit{labels}$[i]$ $\gets s, l_s$ $\sim$  \textit{generator}$()$ 
      \EndFor
      \\\\
      \Comment{\small{Append new $0$ or $1$ samples based on the parity of the labels of recall interval samples}}
      \For{$j = $ \textit{first}, \textit{last}}
        \State append(\textit{sequence}, $s$ $\sim$\textit{generator}$($parity(\textit{labels}$[j])))$
      \EndFor
      \State \textbf{return} \textit{sequence}\Comment{\small{Return full sequence}}
    \EndProcedure
  \end{algorithmic}
\end{algorithm}

\subsubsection{Context-Addressed Dependency Task}
\begin{algorithm}
  \caption{Generative Process for Context-Addressed Dependency Task}\label{pseudoContextAddressed}
  \begin{algorithmic}[1]
    \Procedure{ContextAddressedDependency}{\textit{dataset}}\Comment{\small{Generator for Context-Addressed Dependency}}
      \State $\textit{generator} \gets \text{sample generator for \textit{dataset}}$
      \State ${f_{trans}} \gets \text{\textit{sample transformation} \text{function (e.g. copy, even/odd)}}$
	  \State $\textit{randomSeqLength} \gets \text{length of random sequence}$
      \State $\textit{sequence}, \textit{labels} \gets  \{\}, \{\}$
      \\
      \For{{$i = 1,$ \textit{randomSeqLength}}}  \Comment{\small{Randomly sample from the dataset}}
         \State \textit{sequence}$[i]$, \textit{labels}$[i]$ $\gets s, l_s$ $\sim$  \textit{generator}$()$ 
      \EndFor
      \\
      \State \textit{address} $\gets$ \textit{labels}$[$\textit{randomSeqLength}$]$  \Comment{\small{Use the label of the last random sample as an \textit{address}}}
      \State $ s_{address}\gets$ \textit{sequence}$[address]$  \Comment{\small{Find the sample located in \textit{address}}}
	  \State append(\textit{sequence}, ${f_{trans}}(s_{address})$) \Comment{\small{Append a new sample based on the attended sample}}
      \State \textbf{return} \textit{sequence}\Comment{\small{Return full sequence}}
    \EndProcedure
  \end{algorithmic}
\end{algorithm}

\subsubsection{Stochastic Bouncing Balls Task}
\begin{algorithm}
  \caption{Generative Process for Bouncing Balls Task}\label{pseudoBouncingBalls}
  \begin{algorithmic}[1]
    \Procedure{StochasticBouncingBalls}{}\Comment{\small{Generator for Bouncing Balls}}
      \State $\textit{generator} \gets \text{environment+physics generator}$\Comment{\small{Change ball sprite on collision with walls}}
	  \State $\textit{nBalls} \gets \text{number of balls to simulate}$
	  \State $\textit{seqLength} \gets \text{length of sequence}$
      \\
      \State \textit{sequence}$[1] \gets s \sim$  \textit{generator}$()$  \Comment{\small{Generate initial state with random positions and speed}}
      \For{{$i = 2,$ \textit{seqLength}}}  \Comment{\small{Simulate the next steps}}
         \State \textit{sequence}$[i]$ $\gets s \sim$  \textit{generator}$($\textit{sequence}$[i-1])$ 
      \EndFor
      \\
      \State \textbf{return} \textit{sequence}\Comment{\small{Return full sequence}}
    \EndProcedure
  \end{algorithmic}
\end{algorithm}

\subsection{Additional Results}
\begin{figure}[H]
    \includegraphics[width=\linewidth]{figures/Task1/100/sample50}
    \includegraphics[width=\linewidth]{figures/Task1/60/sample}
    \includegraphics[width=\linewidth]{figures/Task1/50/sample}
    \caption{Additional samples from \emph{IN}-GTM in Perfect Recall Task for different sequence length (top $L=100$, middle $L=60$ with a different recall interval and bottom $L=50$).}
\end{figure}
\begin{figure}[H]
    \includegraphics[width=\linewidth]{figures/Task12/50/sample4}
    \caption{Additional samples from \emph{IN}-GTM in Context-Addressed Dependency Task for $L=50$ sequences.}
\end{figure}
\begin{figure}[H]
    \includegraphics[width=\linewidth]{figures/Task7/50/sample}
    \caption{Additional samples from \emph{IN}-GTM in One-Shot Recall Task for $L=50$ sequences.}
\end{figure}
\begin{figure}[H]
    \includegraphics[width=\linewidth]{figures/EvenOddTrans}
    \caption{Time step to time step transition matrices over MNIST classes obtained from sample sequences produced by \emph{IN}-GTM in Even-Odd Transition Task for $L=50$ sequences. We obtain these transition matrices from sample sequences by first passing each sample through an MNIST classifier ensemble to obtain their class labels. Then, we calculate the transitions between classes in different pairs of time steps. We should see that in the diagonal of the higher level matrix above (e.g. transition matrix between $1$st step and $(L-4)$th step) the classes should transition according to their parity (alternating high probability in $0$ and $1$ columns). In the rest of the higher level matrix (e.g. transition matrix between $1$st step and $(L-3)$th step) we should see a uniform distribution between $0$ and $1$ columns and zero probability in the other columns. Although with some minor imperfections, we can see that the \emph{IN}-GTM successfully recovered the correct transition matrices.}
\end{figure}
